# Supplementary material for: A robust and efficient video representation for action recognition
Source: arXiv:1504.05524 source file (2015-04-21)
Supplement: Supplementary file 1 [file appendix.tex]

\section{Further results}
\label{sec:more-results}

\begin{table*}
    \centering
    \begin{tabular}{|l||ccc||ccc|}
       \hline
                          & \multicolumn{3}{c||}{Drinking}      & \multicolumn{3}{c|}{Smoking}        \\
                          &            &            & Stabilized &            &            & Stabilized \\
                          & Baseline   & Stabilized & w/ hum det & Baseline   & Stabilized & w/ hum det \\
      \hline\hline
          HOG             &      53.74 &      58.39 &      55.51 &      25.34 &      29.56 &      33.22 \\
          HOF             &      81.68 &      79.90 &      82.70 &      29.79 &      36.21 &      30.93 \\
          MBH             &      74.84 &      76.91 &      76.02 &      39.69 &      44.34 &      43.99 \\
      \hline
          HOG$+$HOF       &      80.10 &      79.83 &      77.93 &      32.67 &      33.15 &      33.69 \\
          HOG$+$MBH       &      76.86 &      78.72 &      77.42 &      37.12 &      36.46 &      37.68 \\
          HOF$+$MBH       &      81.99 &      81.47 &      81.35 &      37.33 &      39.20 &      41.26 \\
      \hline
          HOG$+$HOF$+$MBH &      80.78 &      83.47 &      82.77 &      37.86 &      40.80 &      36.44 \\
      \hline\hline
                          & \multicolumn{3}{c||}{Open door}     & \multicolumn{3}{c|}{Sit down}       \\
                          &            &            & Stabilized &            &            & Stabilized \\
                          & Baseline   & Stabilized & w/ hum det & Baseline   & Stabilized & w/ hum det \\
      \hline\hline
          HOG             &      17.07 &      21.64 &      23.11 &      14.98 &      14.94 &      14.32 \\
          HOF             &      17.40 &      22.86 &      24.30 &      24.95 &      24.68 &      25.55 \\
          MBH             &      28.88 &      26.89 &      25.20 &      25.83 &      26.67 &      25.47 \\
      \hline                                                                                      
          HOG$+$HOF       &      17.82 &      27.51 &      28.99 &      23.91 &      25.13 &      25.75 \\
          HOG$+$MBH       &      27.39 &      29.69 &      28.91 &      24.88 &      24.31 &      24.83 \\
          HOF$+$MBH       &      25.86 &      24.71 &      28.70 &      26.58 &      25.83 &      26.70 \\
      \hline                                                                                      
          HOG$+$HOF$+$MBH &      26.92 &      27.53 &      28.88 &      29.49 &      26.12 &      26.67 \\
      \hline
    \end{tabular}
    \caption{Comparison of the stabilization variants (with and without human detector) to the baseline method for the action localization task. We show results on two datasets: the \emph{Coffee \& Cigarettes} dataset and the DLSBP dataset~\citep{Duchenne2009} (actions \emph{Open Door} and \emph{Sit Down}).}
    \label{tab:localization-compare-all-full}
\end{table*}
